# Supplementary material for: Onset of Constituent Quark Number Scaling in Heavy-Ion Collisions at RHIC
Source: arXiv:2504.02531 source file (2025-08-11)
Supplement: Supplementary file 1 [file Supplemental.tex]

\documentclass[twocolumn,aps,prl,floatfix,superscriptaddress]{revtex4-1}

\usepackage{hyperref}
\usepackage[utf8]{inputenc}

\usepackage{graphicx}
\usepackage{dcolumn}
\usepackage{amsmath}
\usepackage{supertabular}
\usepackage{multirow}

\usepackage{color}
\usepackage{cancel}
\usepackage{ulem}
\usepackage{array}
\usepackage{tabularx}

%==========================================================%
%\input{../Common/Include}
%\graphicspath{./Figs_ShortPaper/}
%----------------------------------------------------
\usepackage{amsmath}
\usepackage{amssymb}
\usepackage{xcolor}

%% To remove some words or sentences

%% To add new words or sentencesƒ

%% To add comments

\newcommand {\rootsNN}  {\ensuremath{\sqrt{s_{_{\rm{NN}}}}}}

\usepackage{color}

\usepackage{multirow}

\begin{document}
%\linenumbers

\title{Supplemental Material: Onset of Constituent Quark Number Scaling in Heavy-Ion Collisions at RHIC} 

\bigskip

%%%% _______Author list______and Affiliation________

\input{authorlist_short.tex}
\collaboration{STAR Collaboration}\noaffiliation

\date{\today}
\begin{abstract}
\end{abstract}

\maketitle
\onecolumngrid

\section{Data-model comparsion: $p_T$ dependence of $v_2$}

\begin{figure*}[!htb]
    \centering
    \includegraphics[width=0.95\textwidth]{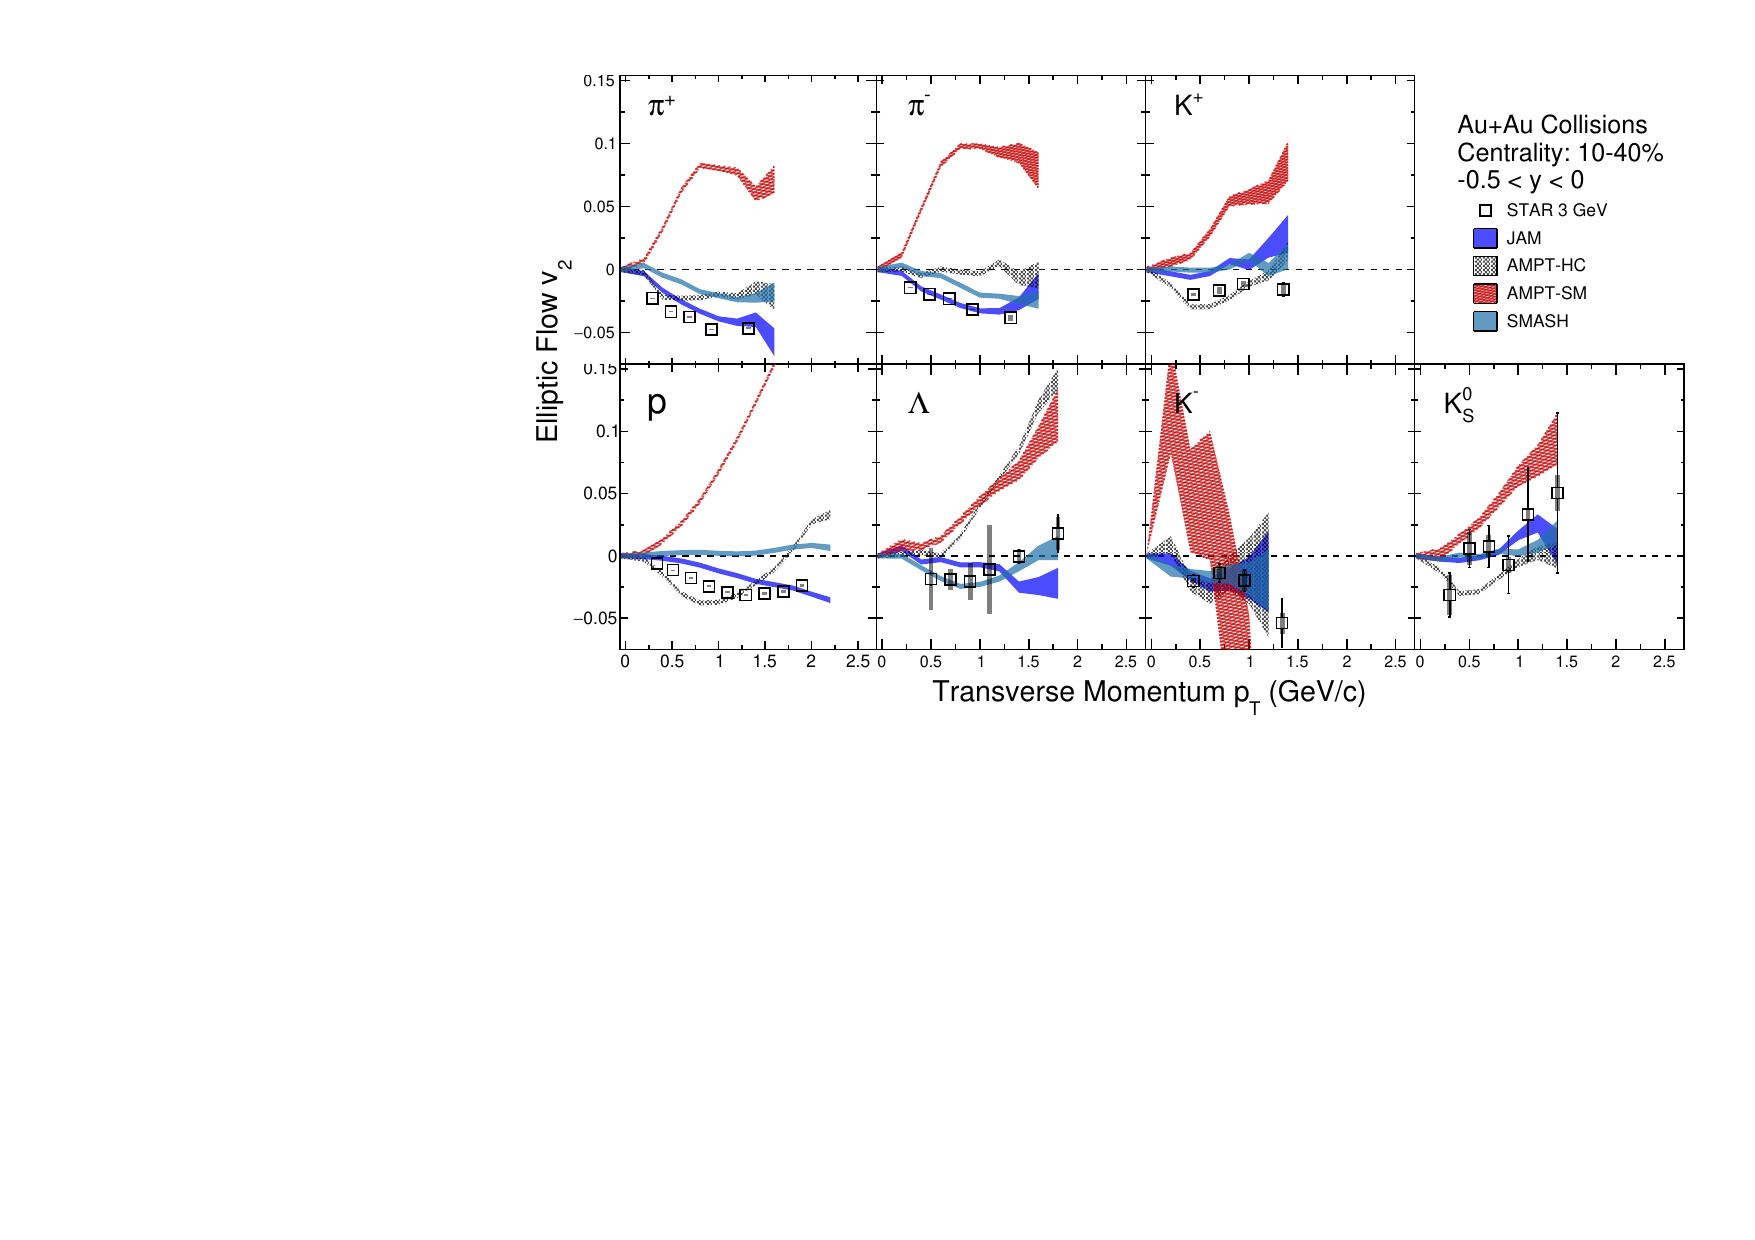}
    \caption{Transverse momentum ($p_T$) dependence of $v_2$ for $\pi^{\pm}$, $K^{\pm}$, $K^{0}_{S}$, $p$, and $\Lambda$ 
    in 10\%--40\% centrality for Au+Au collisions at {\rootsNN} = 3.0 GeV.
    Statistical and systematic uncertainties are shown as bars and bands, respectively. 
    Different bands represent the results from JAM (blue), 
    AMPT-HC (black), AMPT-SM (red), and SMASH (cyan) calculations.
    %$K^-$ calculations from AMPT-SM are not shown due to the rarity of production
    }
    \label{Fig:fig_v2pt_3GeV}
\end{figure*}

Figure \ref{Fig:fig_v2pt_3GeV} presents the $p_T$ dependence of $\pi^{\pm}$, $K^{\pm}$, $K^{0}_{S}$, $p$, and $\Lambda$
in 10\%--40\% centrality for Au+Au collisions at {\rootsNN} = 3.0 GeV. 
Calculations from different models are represented by the bands, where the ``JAM'' means Jet AA Microscopic Transport Model ~\cite{Nara:2021fuu, Nara:2022kbb} with soft Equation Of State (EOS);  
``AMPT-HC'' and ``AMPT-SM'' refer to Hadron Cascade and String Melting mode of the Multi-Phase Transport Model~\cite{PhysRevC.72.064901, Yong:2023uct};
``SMASH'' means Simulating Many Accelerated Strongly interacting Hadrons~\cite{SMASH:2016zqf} with soft EOS. 
The hadronic transport models JAM, AMPT-HC, and SMASH qualitatively describe the $v_2$ data, 
while the multi-phase transport model AMPT-SM (red band) predicts the opposite sign of $v_2$, 
because it does not account for the finite thickness of the incoming nuclei, 
thus missing the potential shadowing effect from spectator nucleons.

\begin{figure*}[!htb]
    \centering
    \includegraphics[width=0.95\textwidth]{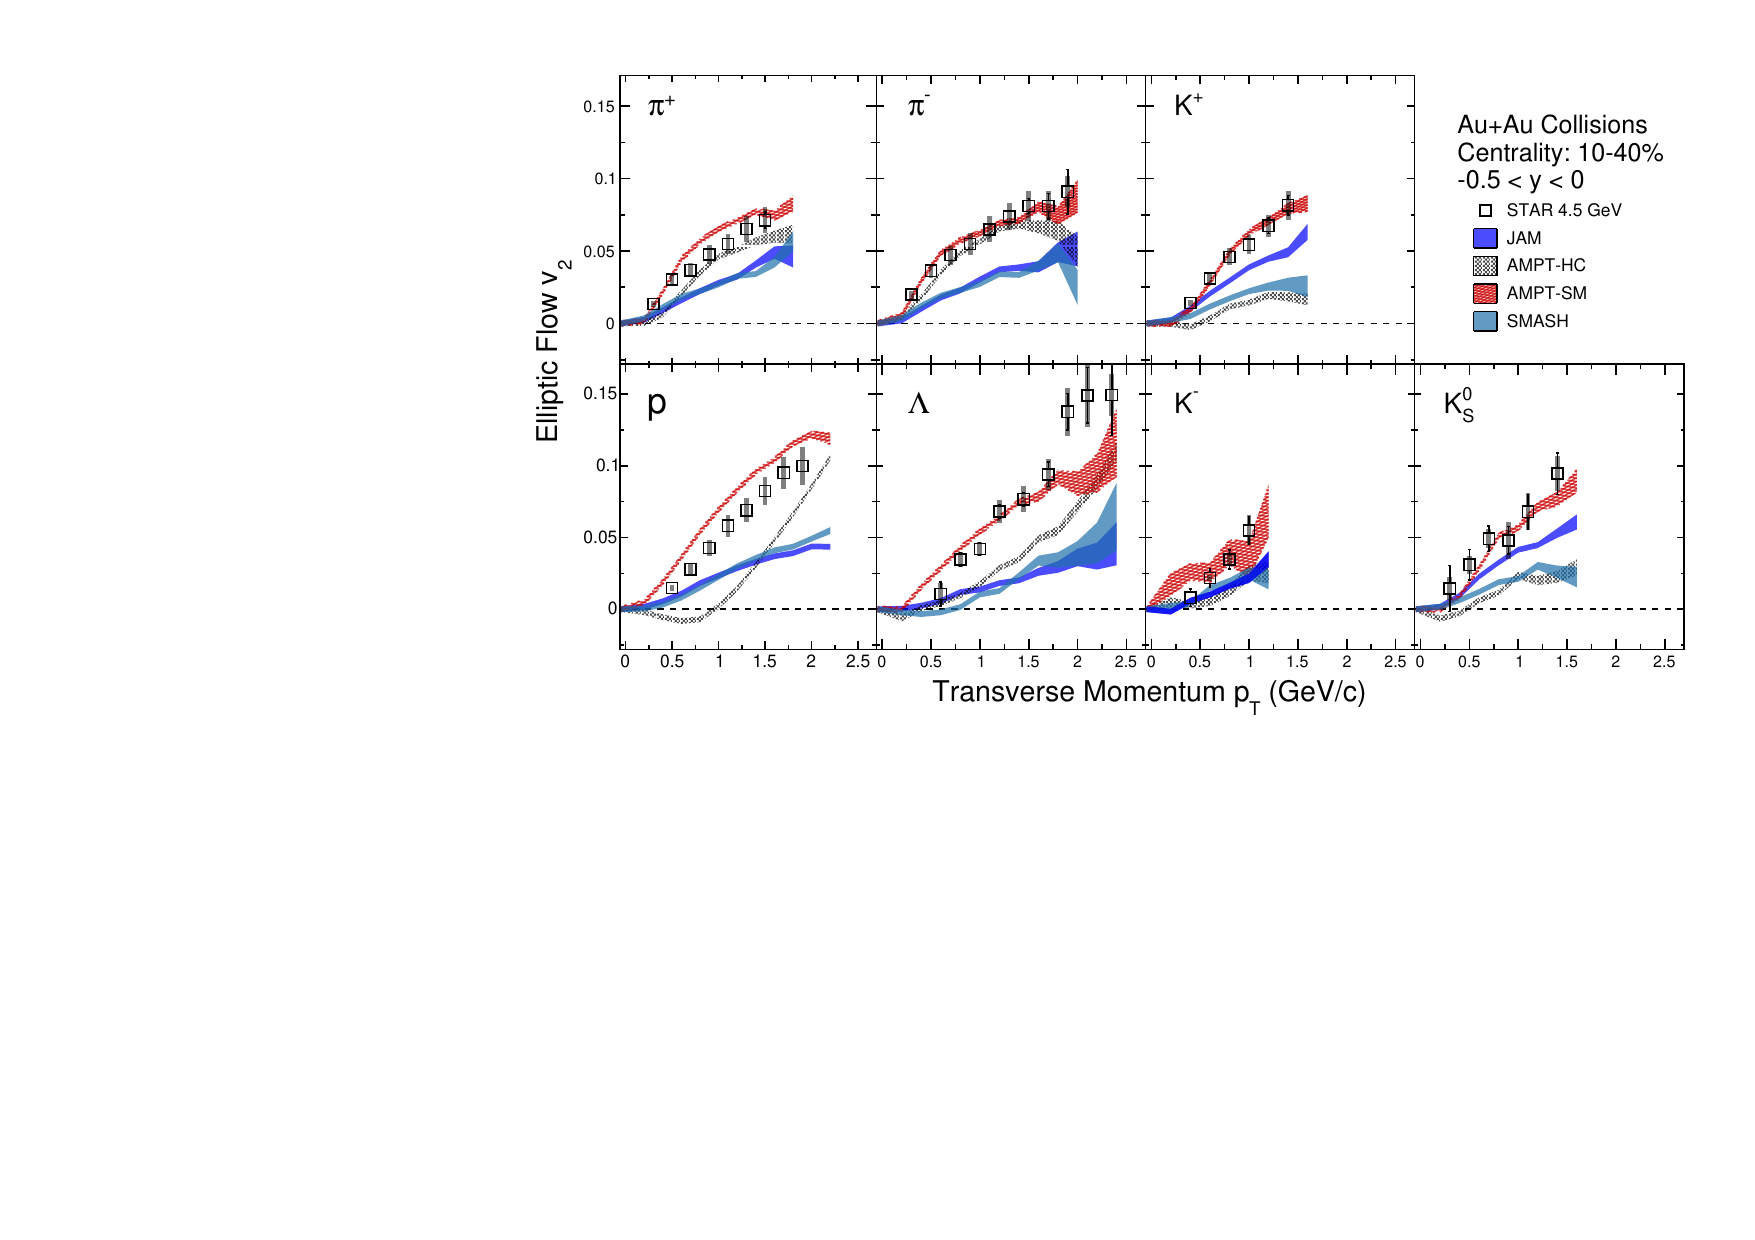}
    \caption{Transverse momentum ($p_T$) dependence of $v_2$ for $\pi^{\pm}$, $K^{\pm}$, $K^{0}_{S}$, $p$, and $\Lambda$ 
    in 10\%--40\% centrality for Au+Au collisions at {\rootsNN} = 4.5 GeV.
    Statistical and systematic uncertainties are shown as bars and bands, respectively. 
    Different bands represent the results from JAM (blue), 
    AMPT-HC (black), AMPT-SM (red), and SMASH (cyan) calculations.
    %$K^-$ calculations from AMPT-SM are not shown due to the rarity of production. 
    }
    \label{Fig:fig_v2pt_4p5GeV}
\end{figure*}

Figure \ref{Fig:fig_v2pt_4p5GeV} shows the $p_T$ dependence of $\pi^{\pm}$, $K^{\pm}$, $K^{0}_{S}$, $p$, and $\Lambda$ 
in 10\%--40\% centrality for Au+Au collisions at {\rootsNN} = 4.5 GeV. 
The hadronic transport models generally underestimate the $v_2$ data (except $\pi^{\pm}$ from AMPT-HC); 
in contrast, AMPT string melting mode better describes the $v_2$ data.
%This suggests that parton interactions play an important role in generating such a significant $v_2$ signal.

\section{Number of Constituent Quarks scaling: $v_{2}/n_{q}$ vs. $p_{T}/n_{q}$}

\begin{figure*}[!htb]
    \centering
    \includegraphics[width=0.95\textwidth]{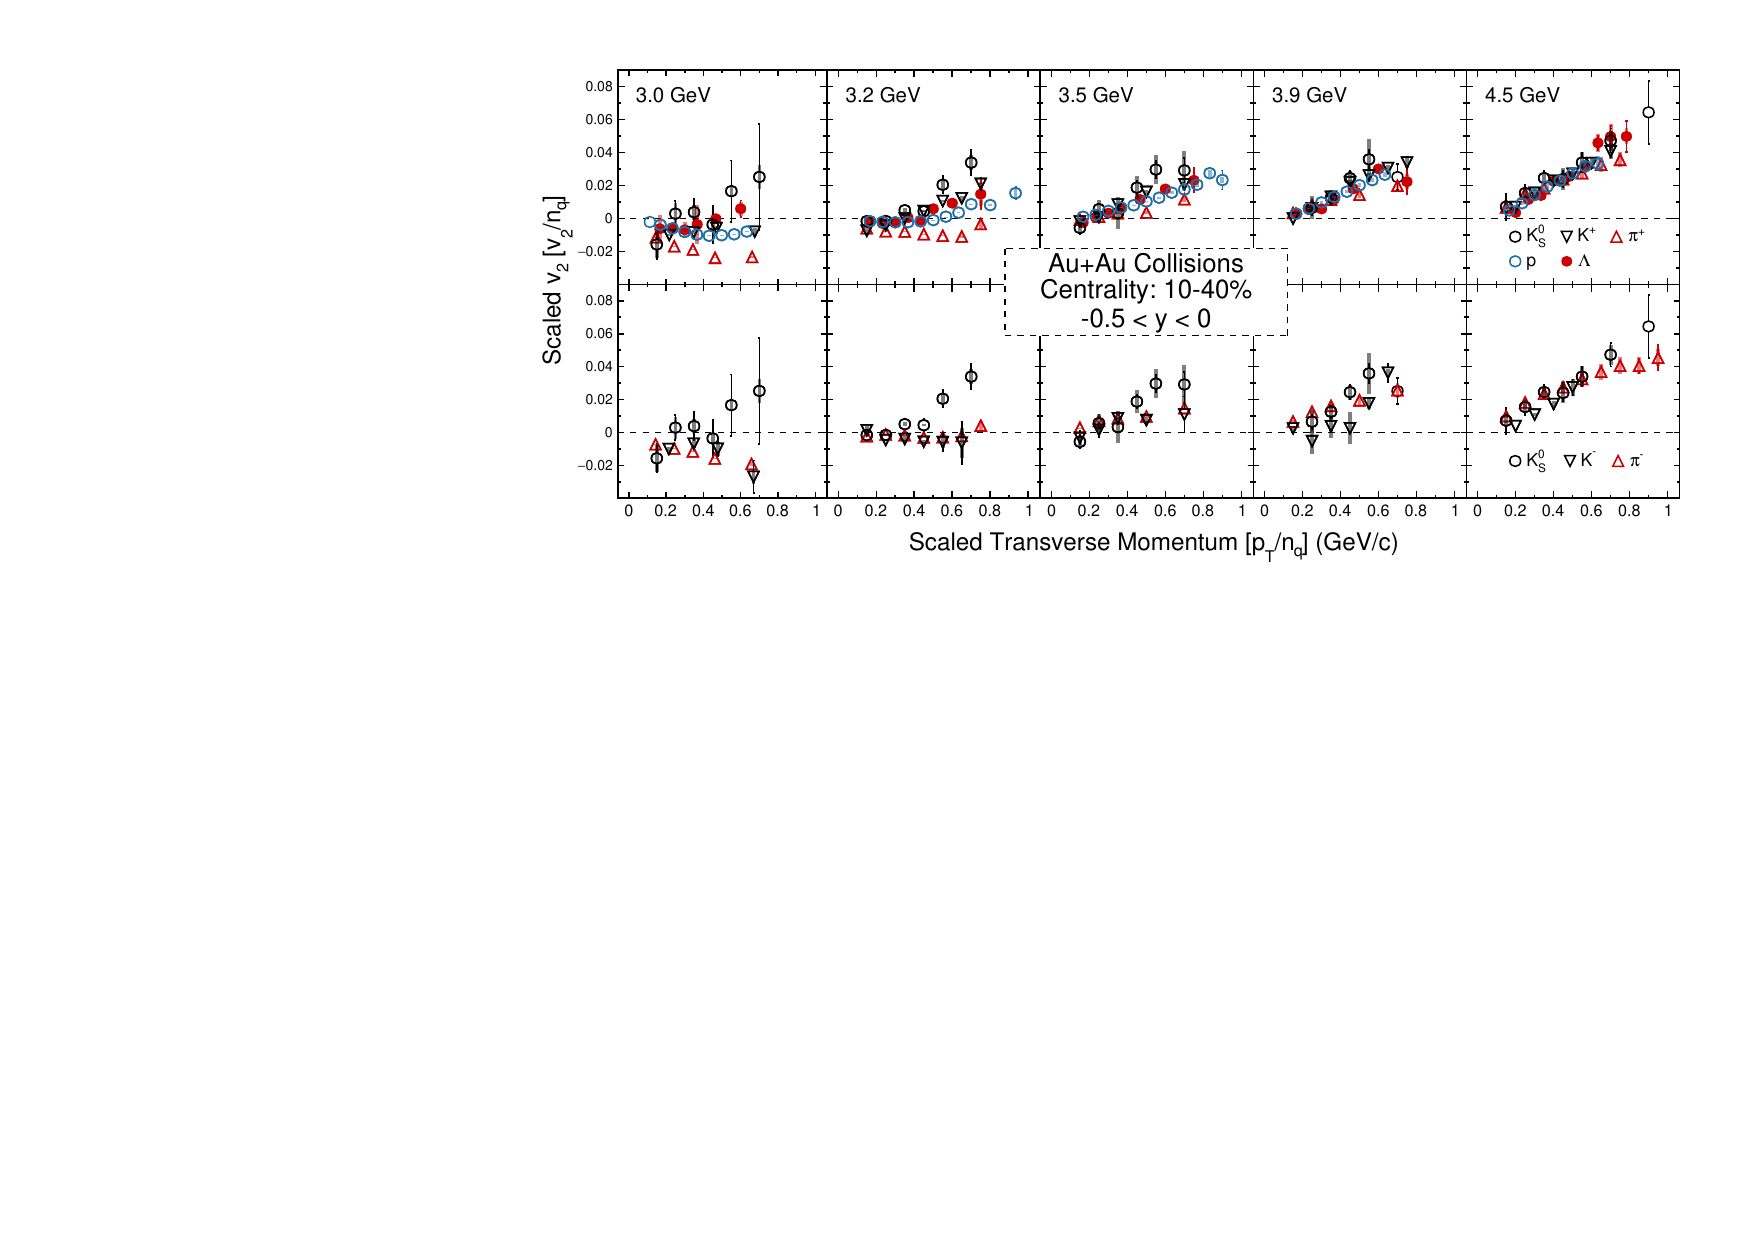}
    \caption{The number of constituent quarks $n_q$ scaled $v_2$ as a function of $n_q$ scaled transverse momentum for particles (upper panel) and anti-particles (lower panel) in 10\%--40\% centrality for Au+Au collisions at {\rootsNN} = 3.0, 3.2, 3.5, 3.9, and 4.5 GeV. }
    \label{Fig:fig_NCQ_pT_nq}
\end{figure*}

Figure \ref{Fig:fig_NCQ_pT_nq} represents the number of constituent quarks $n_q$ scaled $v_2$ as a function of $n_q$ scaled $p_T$
for particles and anti-particles separately in 10\%--40\% centrality for Au+Au collisions.
The $p_{T}/n_{q}$ scaling exhibits better performance than $(m_T - m_0)/n_q$ scaling for $\pi^{\pm}$,
suggesting that the $\pi^{\pm}$ deviation on $(m_T - m_0)/n_q$ scaling at 4.5 GeV, may primarily be attributed to the significantly smaller mass of pions compared to other hadrons.
%This finding is also consistent with the predictions from the original papers that proposed $p_T$-based scaling
Notably, the original NCQ scaling was proposed based on $p_T$~\cite{Molnar:2003ff, Voloshin:2005up}.

\begin{figure*}[!htb]
  \centering   
  \includegraphics[width=0.47\columnwidth]{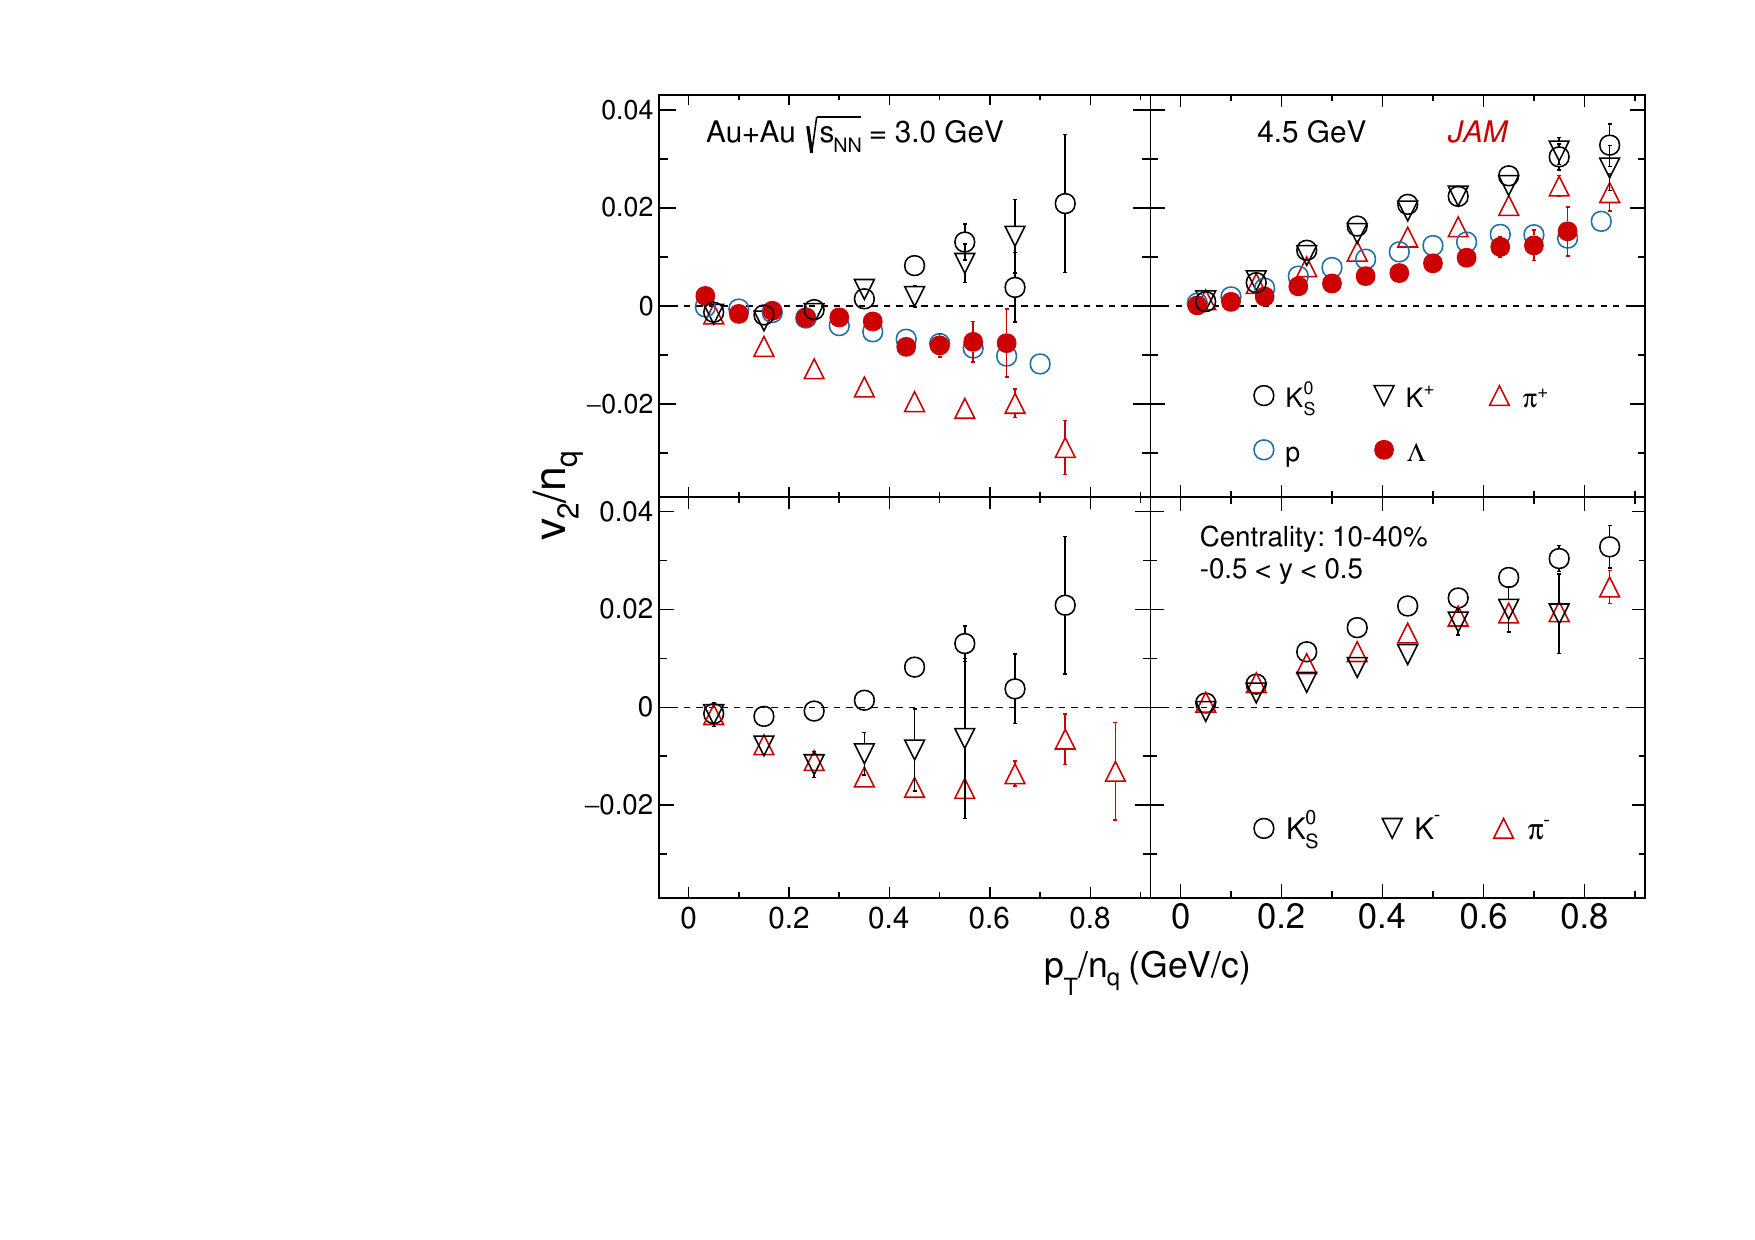}
  \includegraphics[width=0.47\columnwidth]{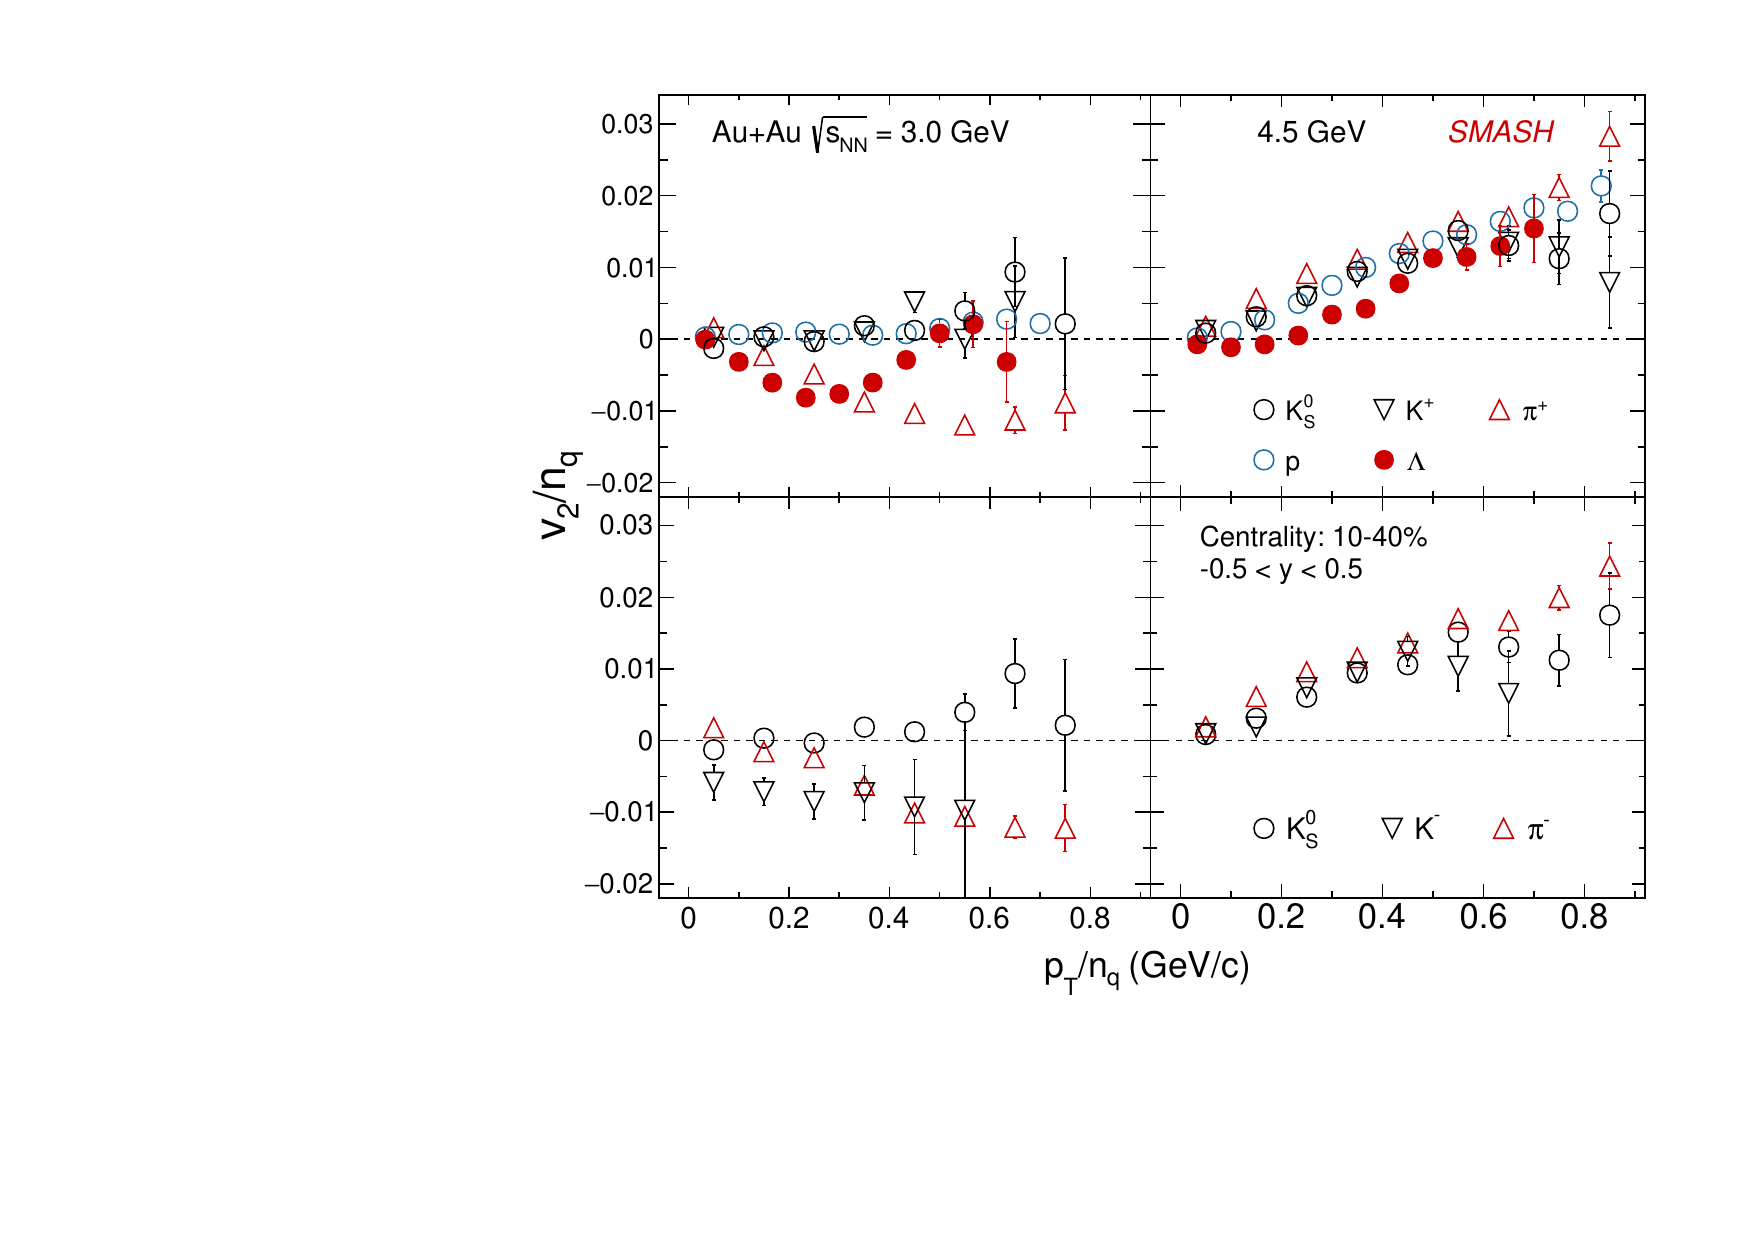}   
  \includegraphics[width=0.47\columnwidth]{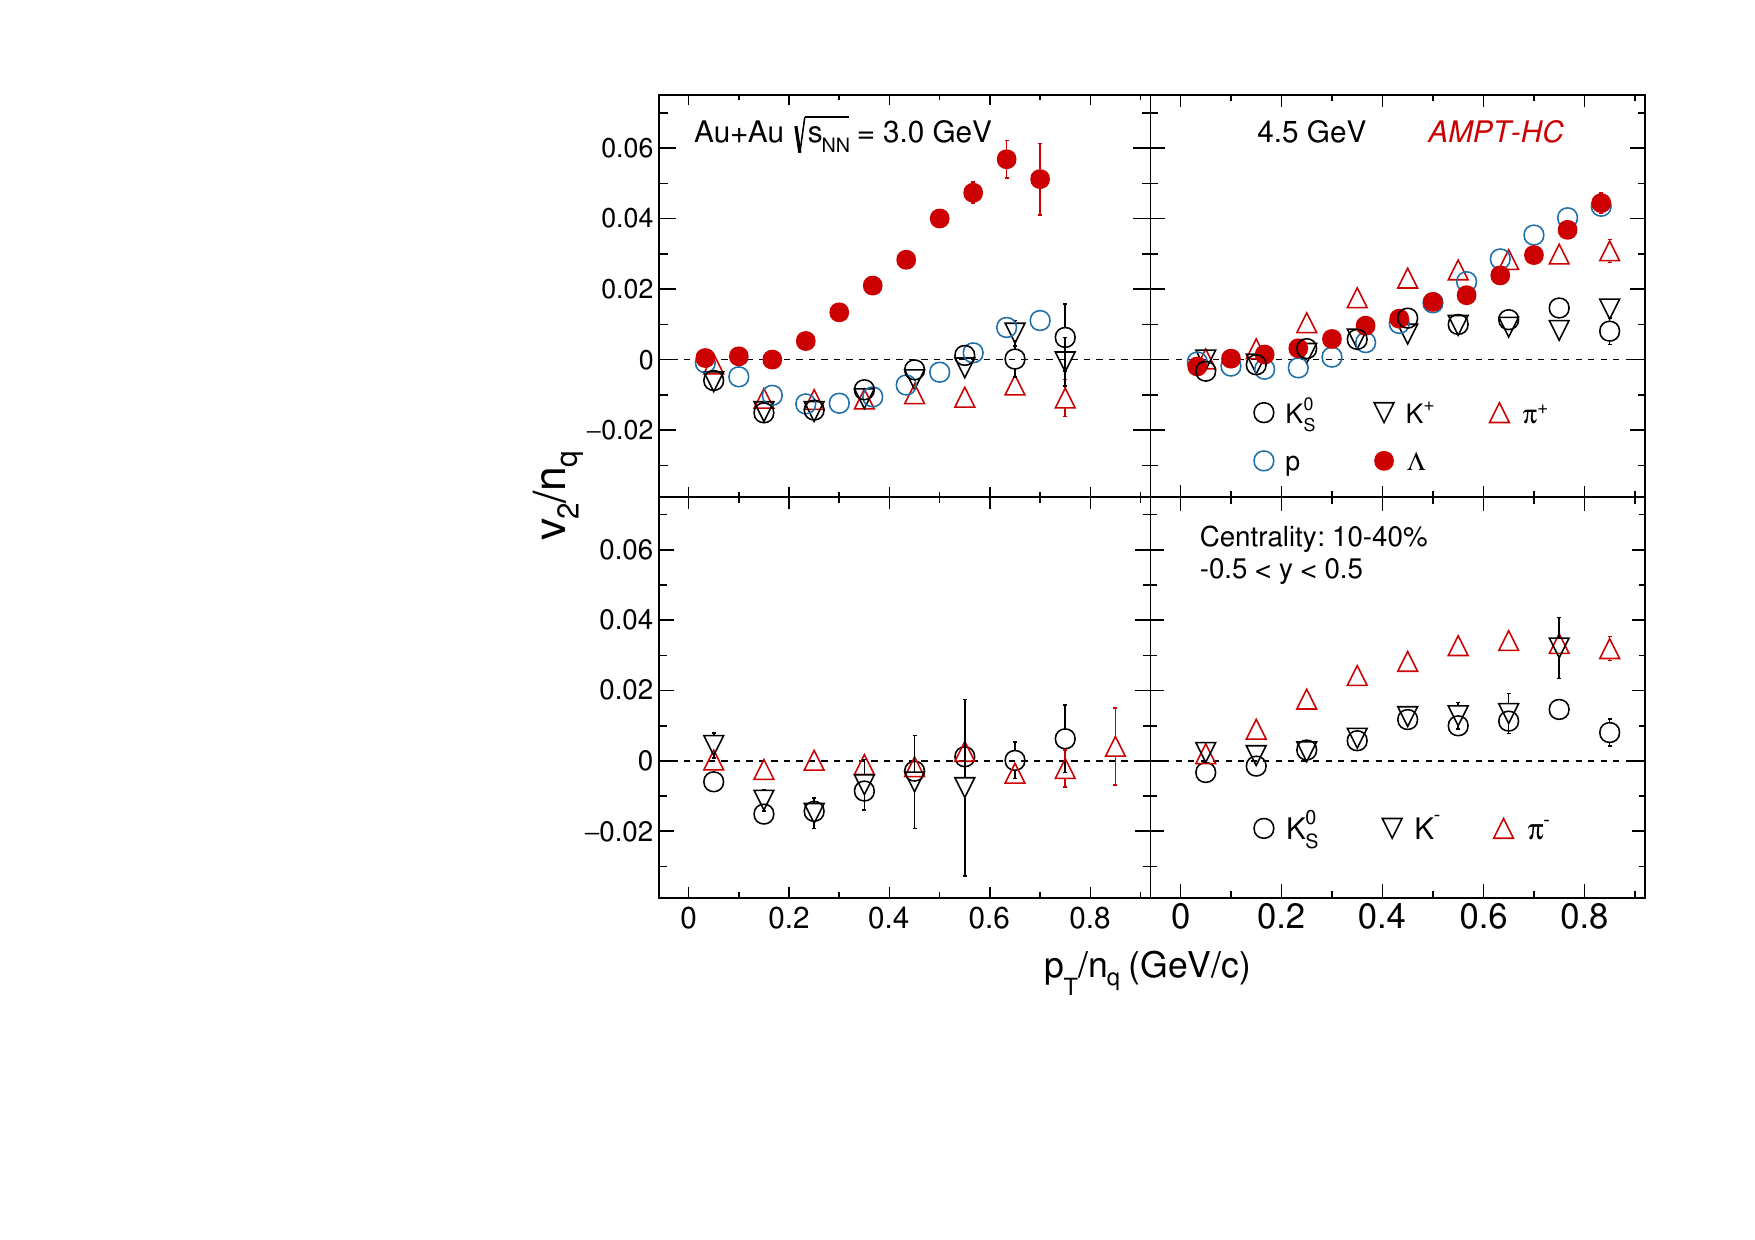}
  \includegraphics[width=0.47\columnwidth]{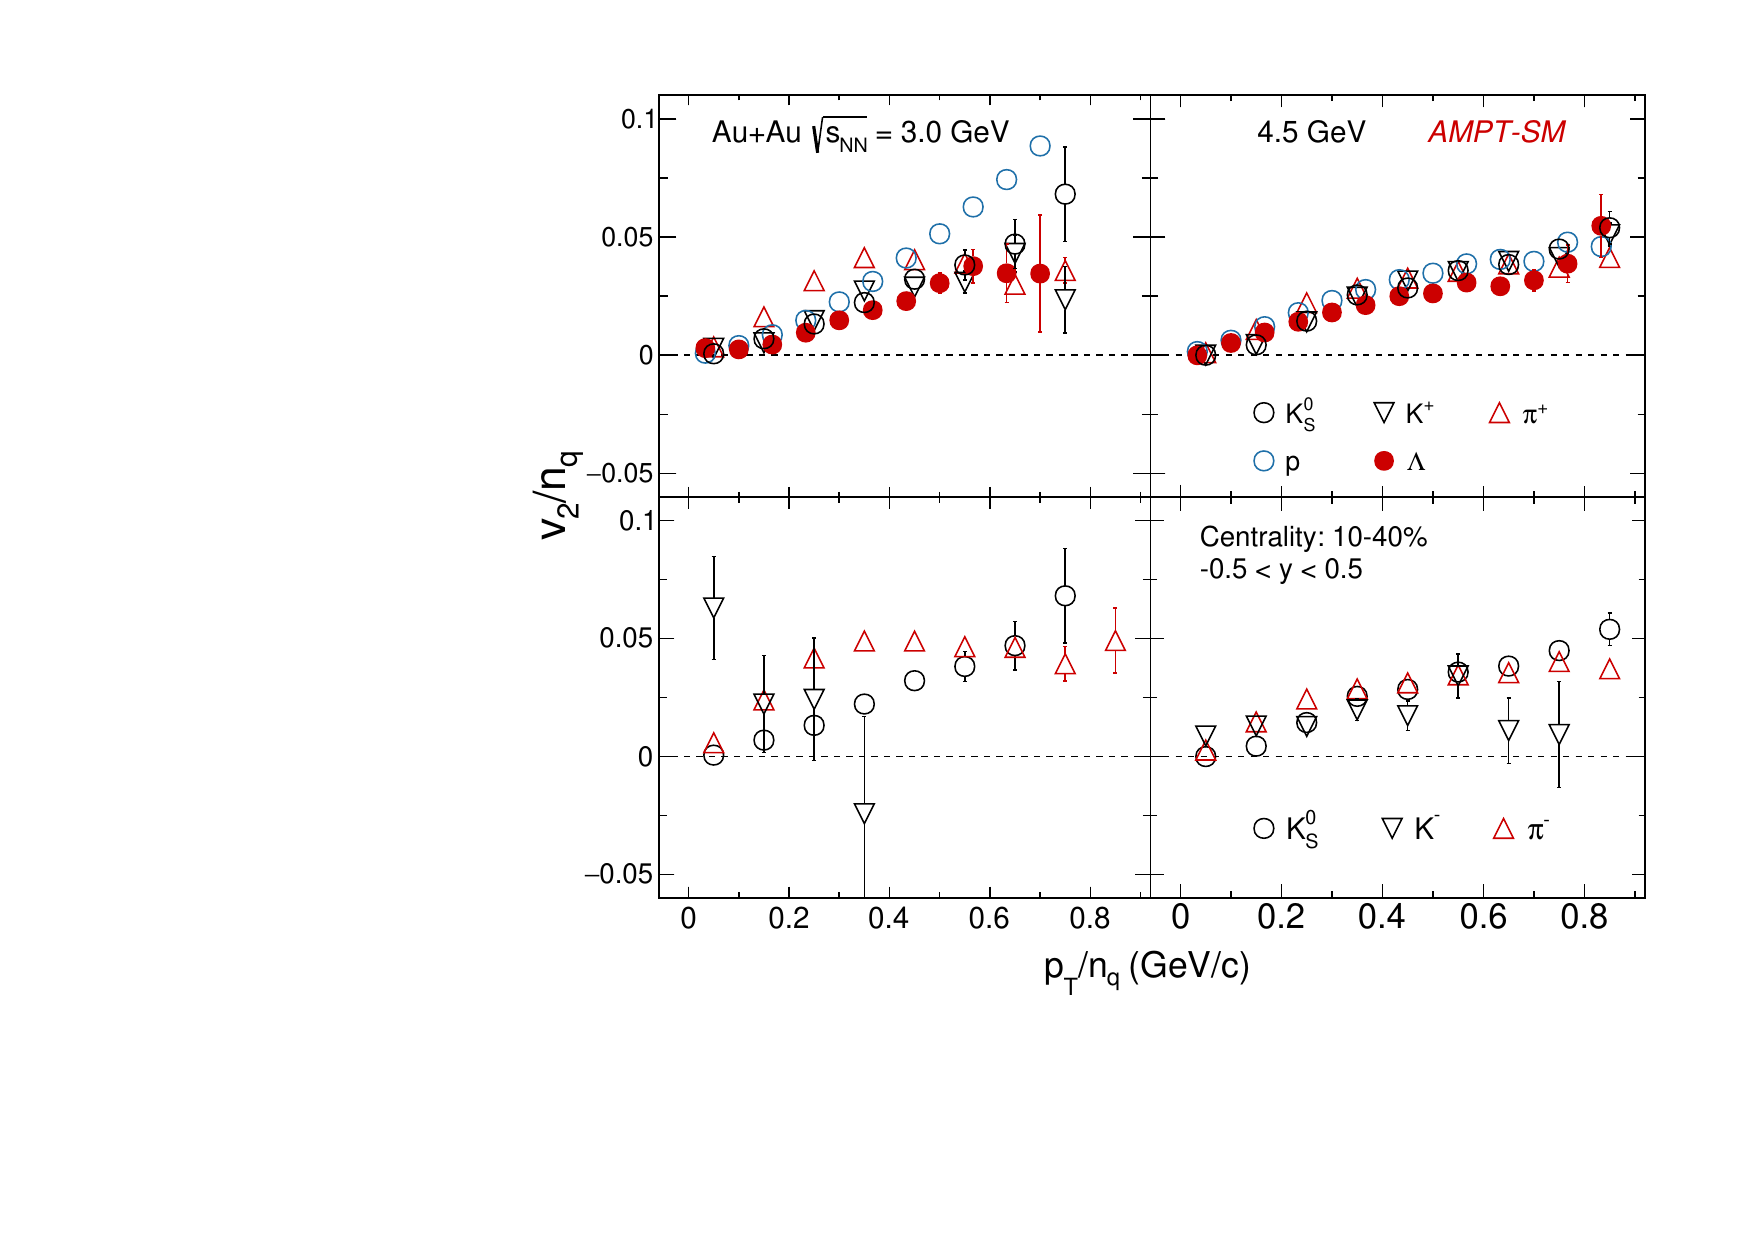}   
    \caption{The number of constituent quarks $n_q$ scaled $v_2$ as a function of $n_q$ scaled transverse momentum in 10\%--40\% centrality for Au+Au collisions at {\rootsNN} = 3.0 and 4.5 GeV from model calculations using JAM, SMASH, AMPT-HC, and AMPT-SM.}
    \label{Fig:fig_NCQ_model}
\end{figure*}

Figure~\ref{Fig:fig_NCQ_model} shows the number of constituent quarks $n_q$ scaled $v_2$ for 
$\pi^{\pm}$, $K^{\pm}$, $K^{0}_{S}$, $p$, and $\Lambda$  in 10\%--40\% centrality at Au+Au collisions {\rootsNN} = 3.0 and 4.5 GeV 
from model calculations using JAM, SMASH, AMPT-HC, and AMPT-SM.
JAM model well captures the NCQ scaling broken at 3.0 GeV, but no scaling is observed at 4.5 GeV.
This may be attributed to JAM being a purely hadronic transport model, where only hadronic interactions are included during the medium evolution.
SMASH and AMPT-HC partially describe the $v_2$ data at 3 GeV. However, SMASH greatly underestimates $v_2$ at 4.5 GeV as shown in Fig.~\ref{Fig:fig_v2pt_4p5GeV}, and AMPT-HC shows a larger deviation from NCQ scaling at the same energy.
In the multi-phase transport model, the HC mode better reproduces the data at 3.0 GeV. 
However, at 4.5 GeV, the SM mode exhibits better NCQ scaling, suggesting that the inclusion of partonic interactions significantly play a key role in enhancing the scaling behavior.

%\section*{Acknowledgments}
%\vspace{10cm}

%\bibliographystyle{unsrt} 
\bibliography{example} % Produces the bibliography via BibTeX.

\end{document}
